# Supplementary material for: Additive-Effect Assisted Learning
Source: arXiv:2405.08235 source file (2024-05-13)
Supplement: Supplementary file 1 [file ridgeTestingPV_testSetting_H0_betasetting_1_Xdist_uniform_sig_0.9_fixedU_TRUE_Lapscale_0.1.pdf]

Setting 1,  $n=200$ ,  $\rho = 0.9$ ,  $lap(0.1)$

Sample Quantiles

t=1

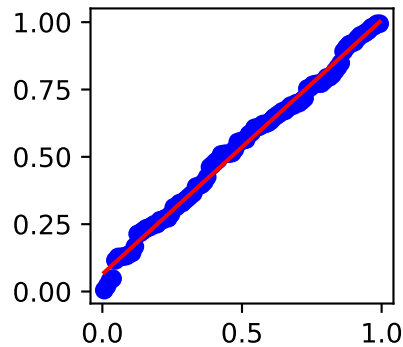

t=2

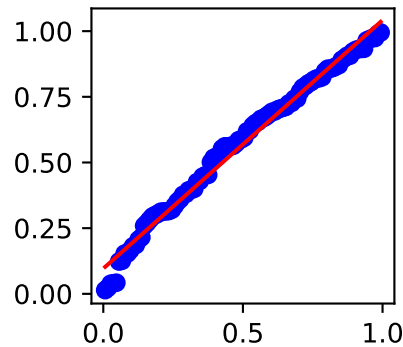

t=3

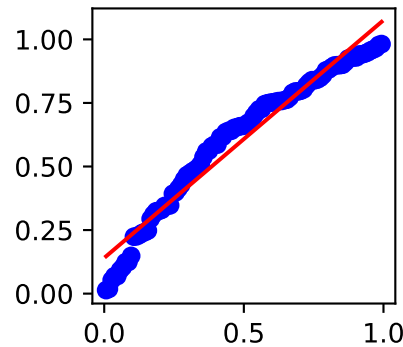

t=4

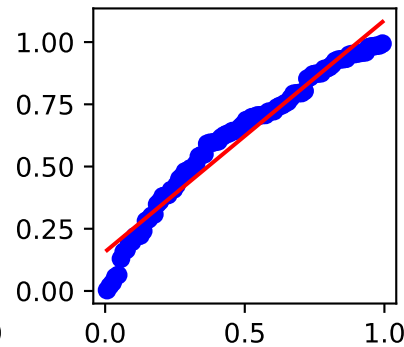

t=5

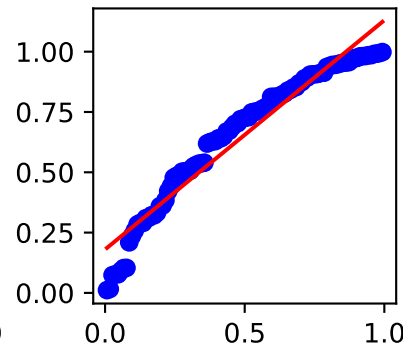

Theoretical Quantiles

Setting 1,  $n=2000$ ,  $\rho = 0.9$ ,  $lap(0.1)$

Sample Quantiles

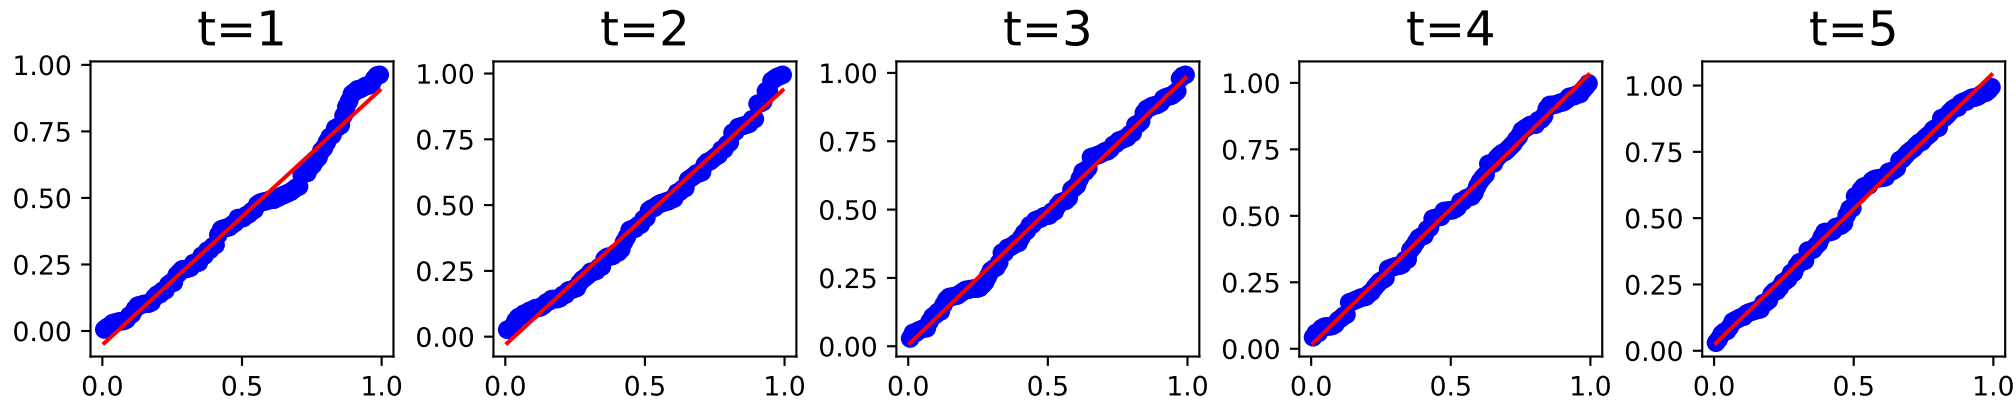

Theoretical Quantiles
